# Supplementary material for: Bringing Masked Autoencoders Explicit Contrastive Properties for Point Cloud Self-Supervised Learning
Source: arXiv:2407.05862 source file (2024-07-08)
Supplement: Supplementary file 1 [file appendix_comparison.tex]

\begin{table}[h!]
	\caption{Comparison to supervised cross-modal 3D representation learning method on ScanObjectNN. Overall accuracy, \ie, OA (\%) is reported.} \label{tab:comparison_supversied}
	\centering
	\begin{tabular}{lccc}
		\toprule[0.95pt]
		Method & Backbone &\#Params (M) & OA (\%)$\uparrow$\\
		\midrule[0.6pt]
		P2P~\citep{P2P} & ResNet101 & 42.7 & 87.4\\
		P2P~\citep{P2P} & HorNet & 195.8 & 89.3\\
		\rowcolor{linecolor} ACT (Ours) & Transformer & 22.1 & 88.2\\
		\bottomrule[0.95pt]
	\end{tabular}
\end{table}
